# Supplementary material for: Toward Artificial Open-Ended Evolution within Lenia using Quality-Diversity
Source: arXiv:2406.04235 source file (2024-06-06)
Supplement: Supplementary file 1 [file 1_supplementary-results.tex]

\newpage
\section{Supplementary Results}
%
% \begin{figure*}[h!]
%     \centering
%     \includegraphics[width=\textwidth]{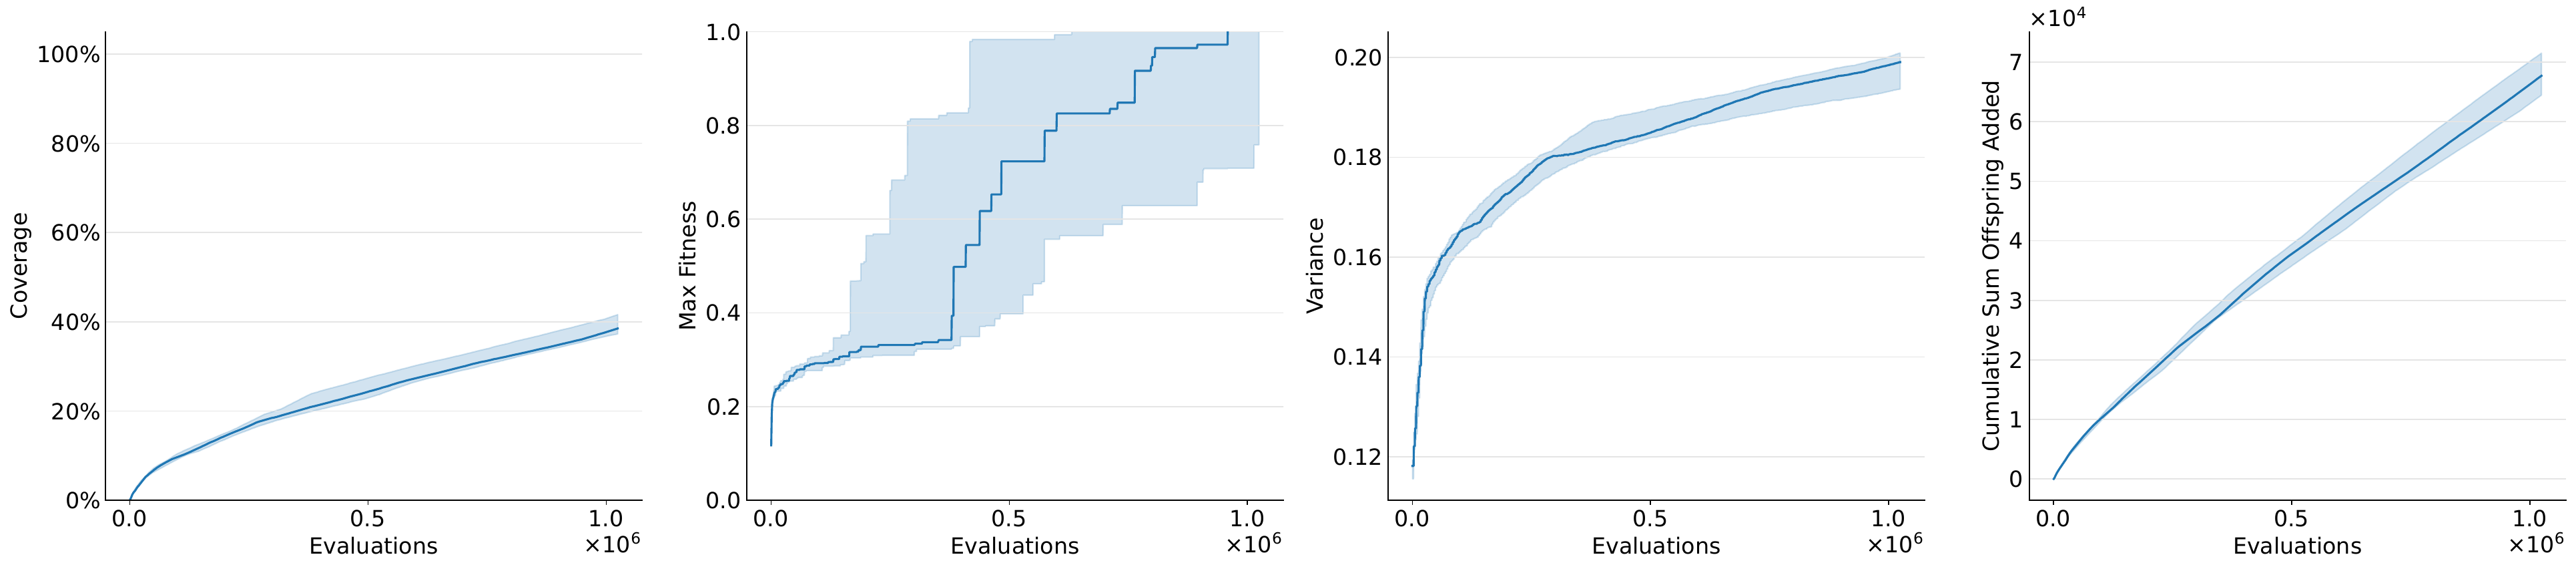}
%     \caption{Entropy, Variance and Cumulative Sum of Offspring Added to the unstructured repertoire for \aurora{} with different fitness functions, including the unsupervised fitness. Each experiment is replicated 20 times with random seeds. The solid line is the median and the shaded area represents the first and third quartiles.}
% \end{figure*}
%
\begin{figure*}[h!]
    \centering
    \includegraphics[width=\textwidth]{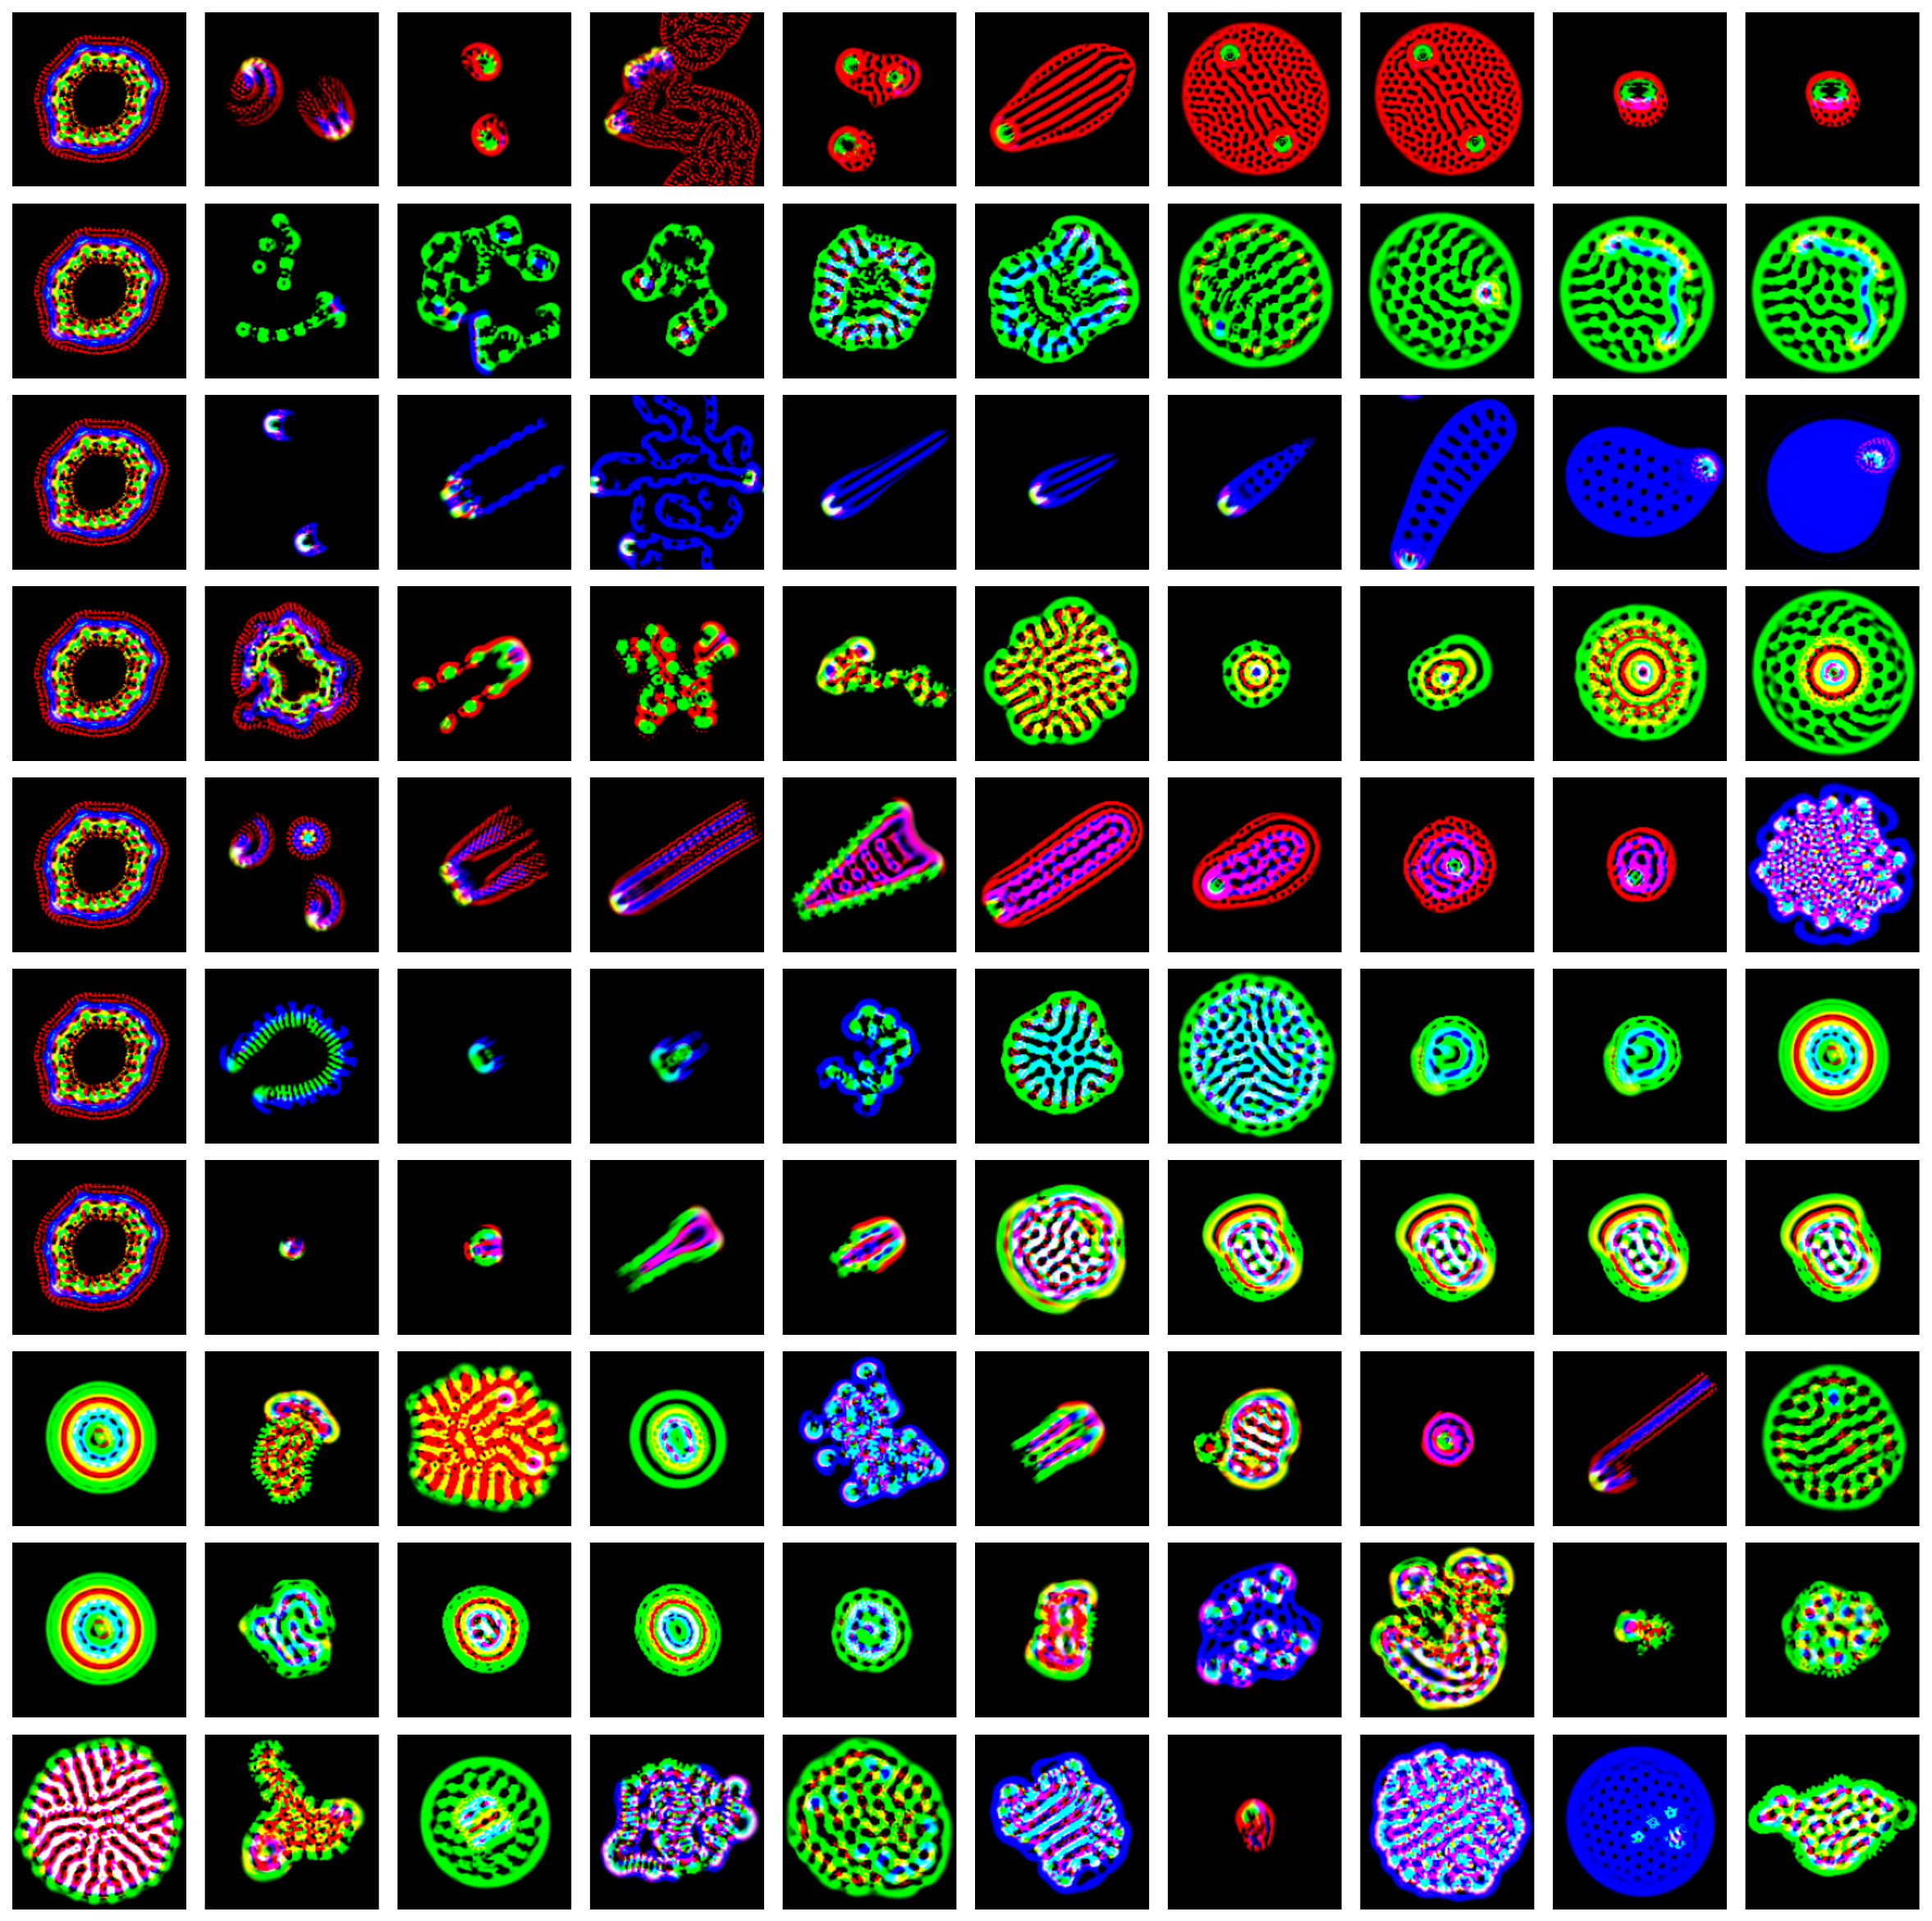}
    \caption{Entropy, Variance and Cumulative Sum of Offspring Added to the unstructured repertoire for \aurora{} with different fitness functions, including the unsupervised fitness. Each experiment is replicated 20 times with random seeds. The solid line is the median and the shaded area represents the first and third quartiles.}
\end{figure*}

% \begin{figure*}[h!]
%     \centering
%     \includegraphics[width=\textwidth]{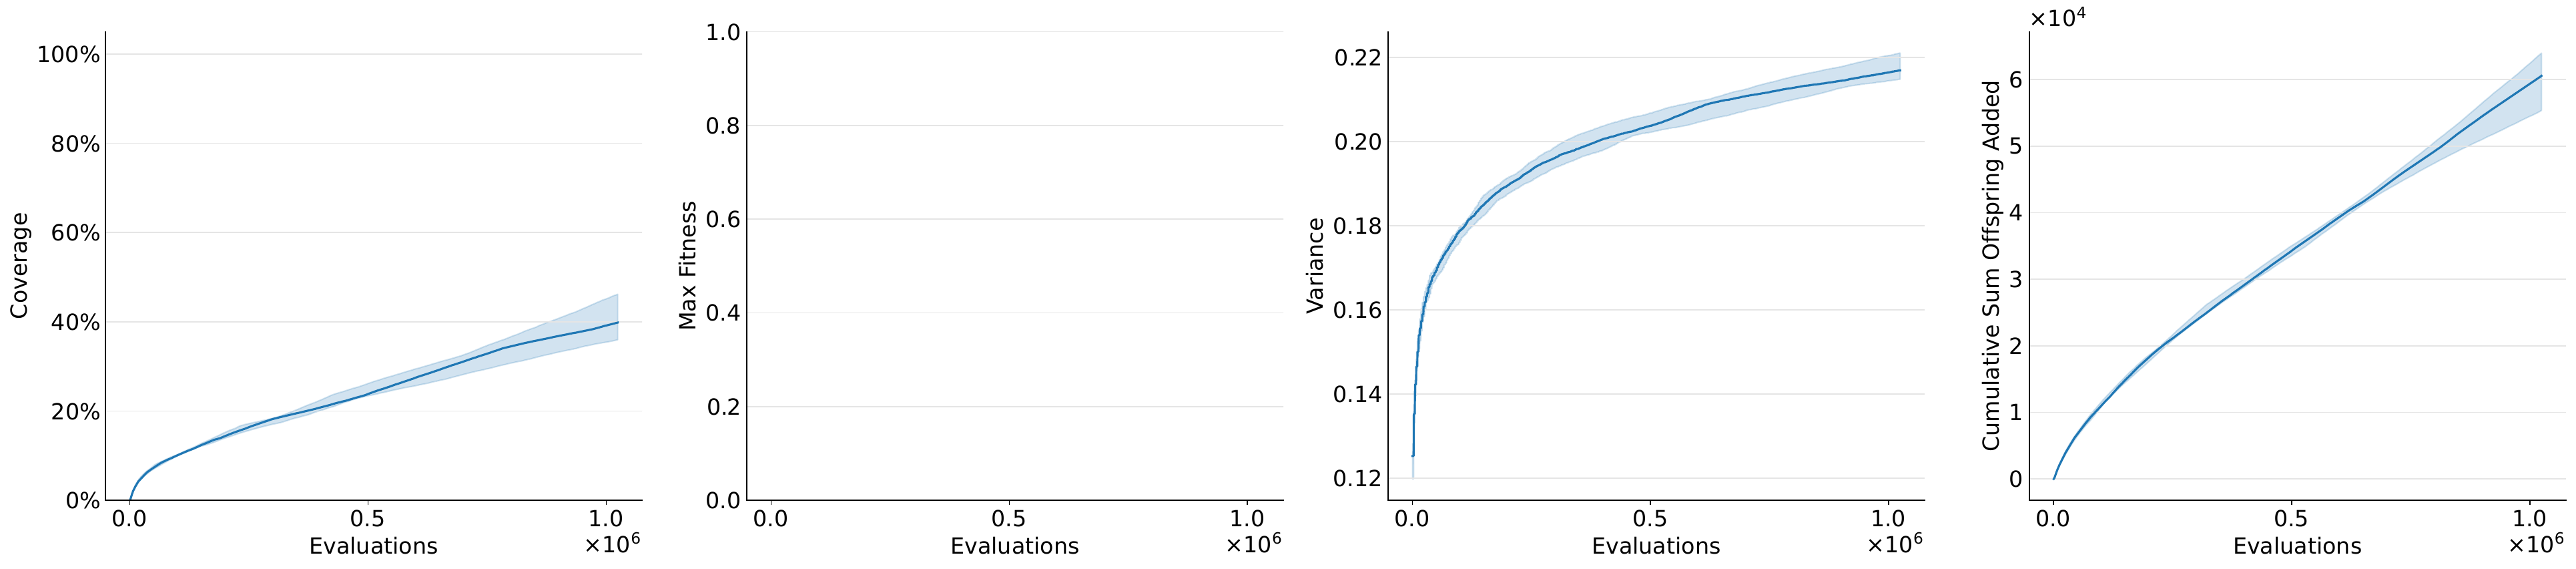}
%     \caption{Entropy, Variance and Cumulative Sum of Offspring Added to the unstructured repertoire for \aurora{} with different fitness functions, including the unsupervised fitness. Each experiment is replicated 20 times with random seeds. The solid line is the median and the shaded area represents the first and third quartiles.}
% \end{figure*}
%
\begin{figure*}[h!]
    \centering
    \includegraphics[width=\textwidth]{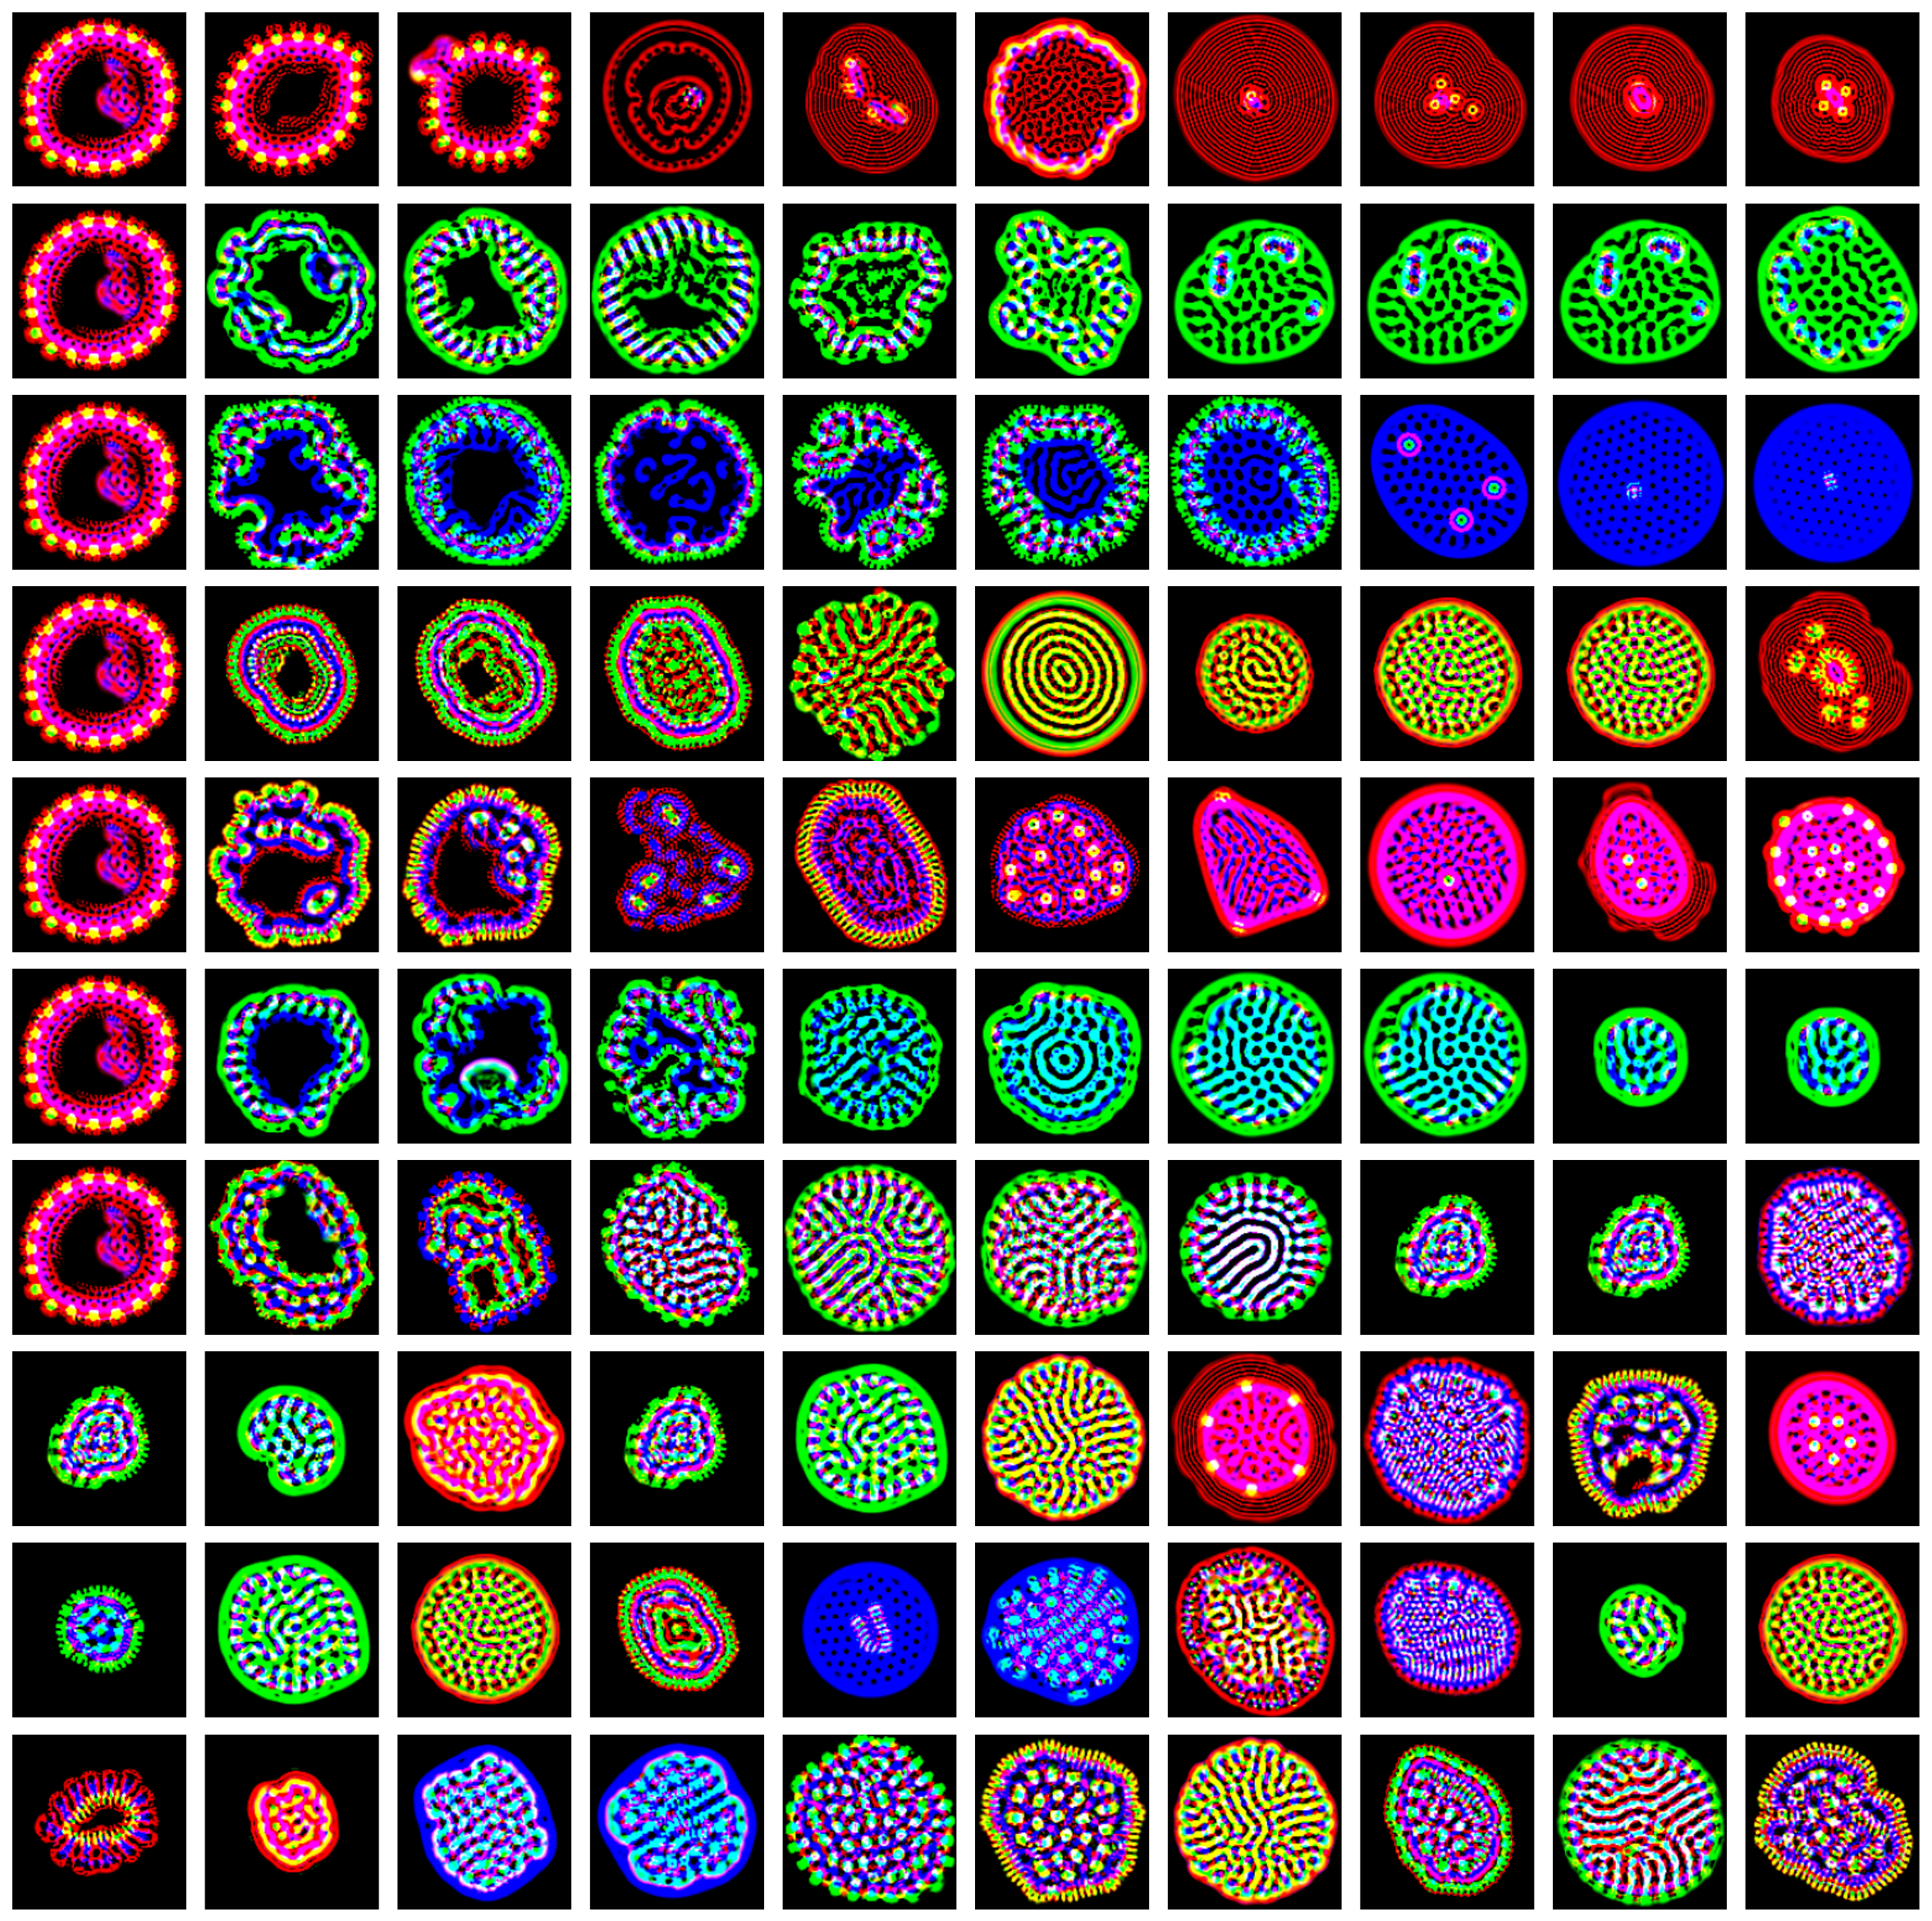}
    \caption{Entropy, Variance and Cumulative Sum of Offspring Added to the unstructured repertoire for \aurora{} with different fitness functions, including the unsupervised fitness. Each experiment is replicated 20 times with random seeds. The solid line is the median and the shaded area represents the first and third quartiles.}
\end{figure*}

% \begin{figure*}[h!]
%     \centering
%     \includegraphics[width=\textwidth]{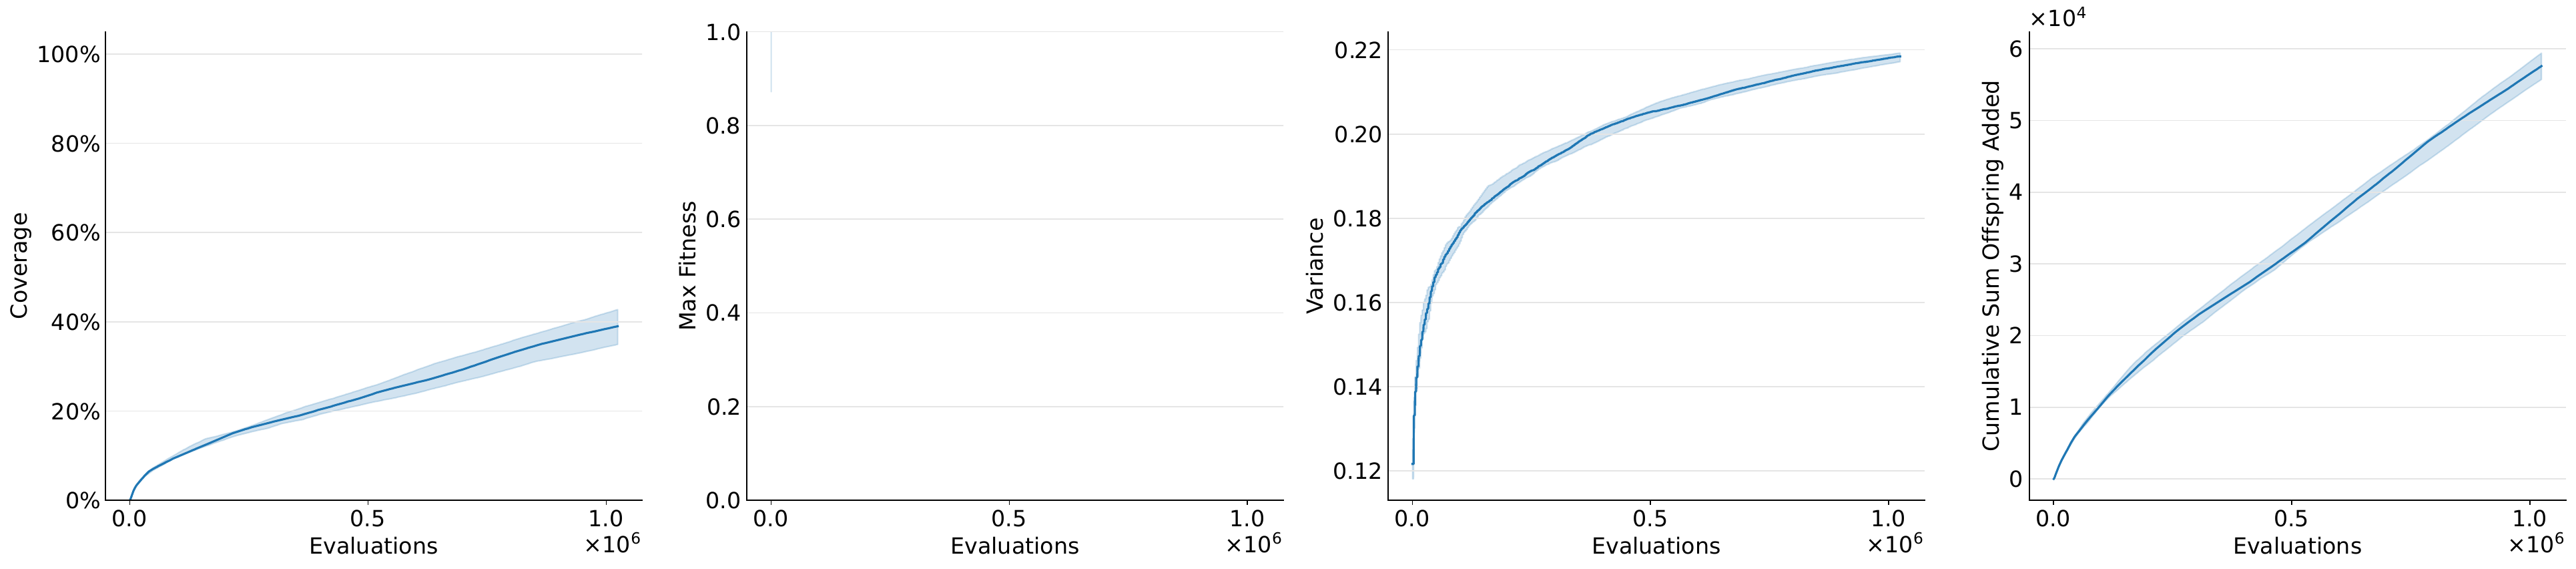}
%     \caption{Entropy, Variance and Cumulative Sum of Offspring Added to the unstructured repertoire for \aurora{} with different fitness functions, including the unsupervised fitness. Each experiment is replicated 20 times with random seeds. The solid line is the median and the shaded area represents the first and third quartiles.}
% \end{figure*}
%
\begin{figure*}[h!]
    \centering
    \includegraphics[width=\textwidth]{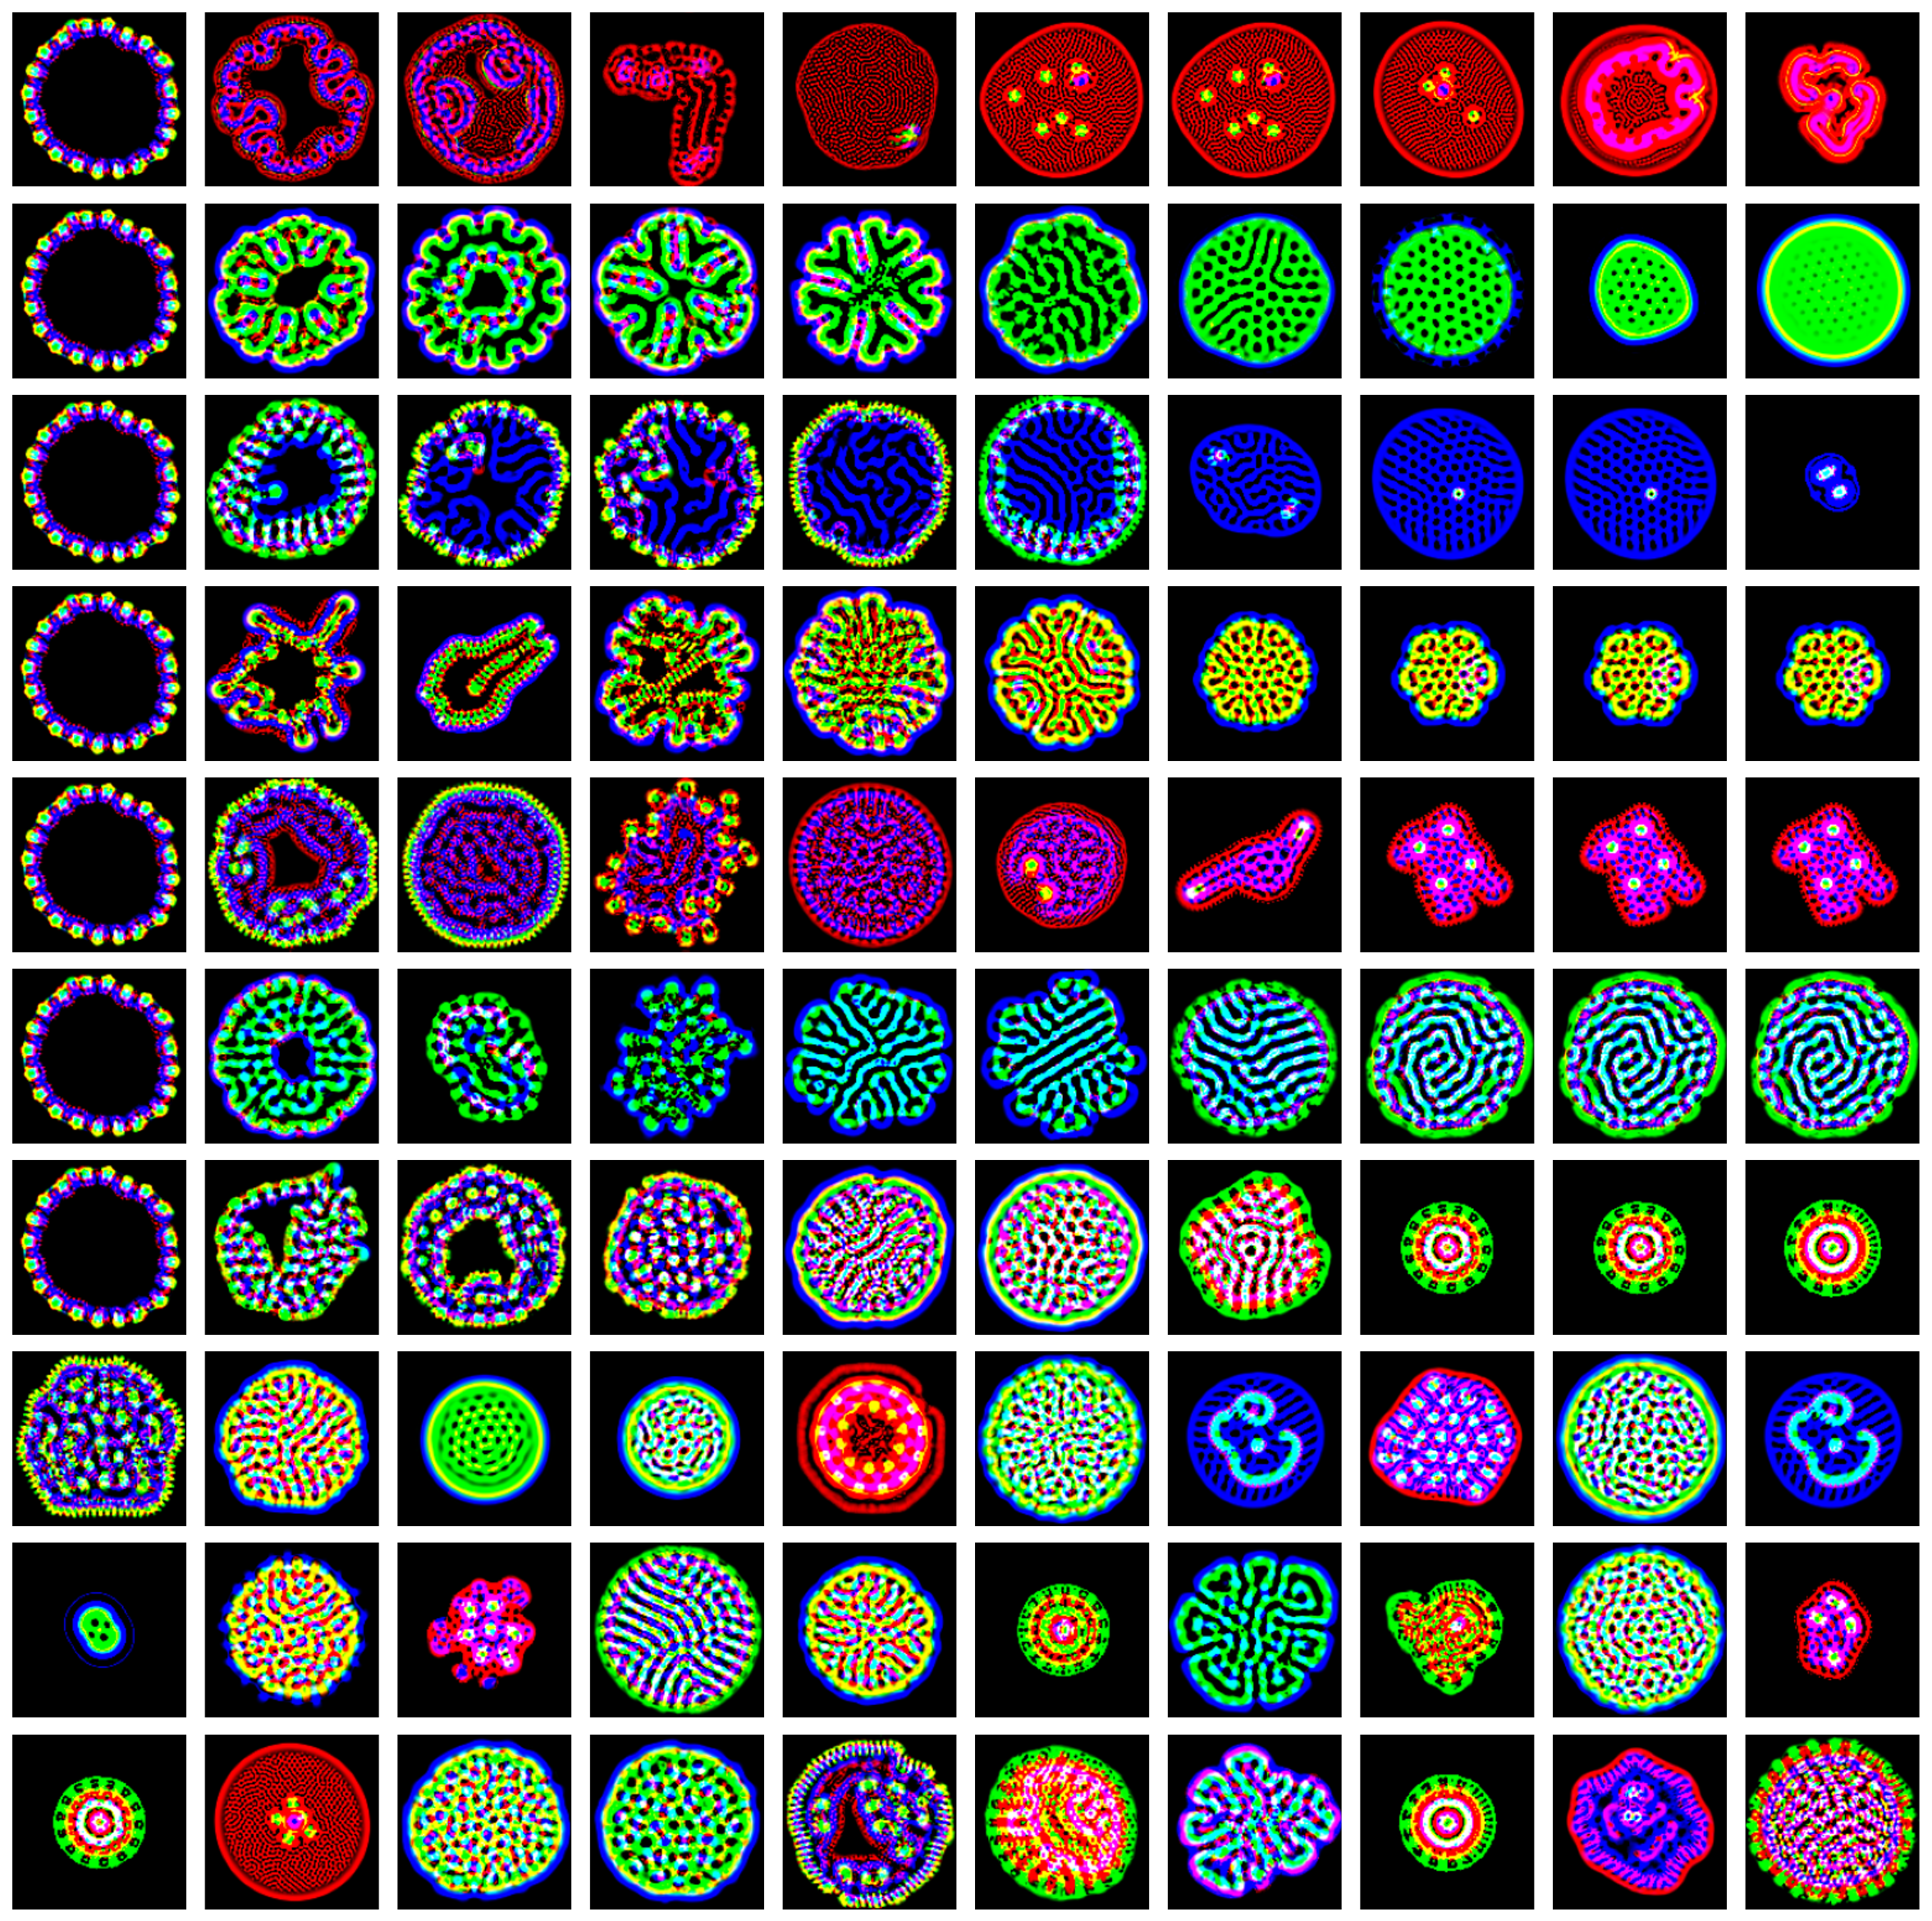}
    \caption{Entropy, Variance and Cumulative Sum of Offspring Added to the unstructured repertoire for \aurora{} with different fitness functions, including the unsupervised fitness. Each experiment is replicated 20 times with random seeds. The solid line is the median and the shaded area represents the first and third quartiles.}
\end{figure*}

% \begin{figure*}[h!]
%     \centering
%     \includegraphics[width=\textwidth]{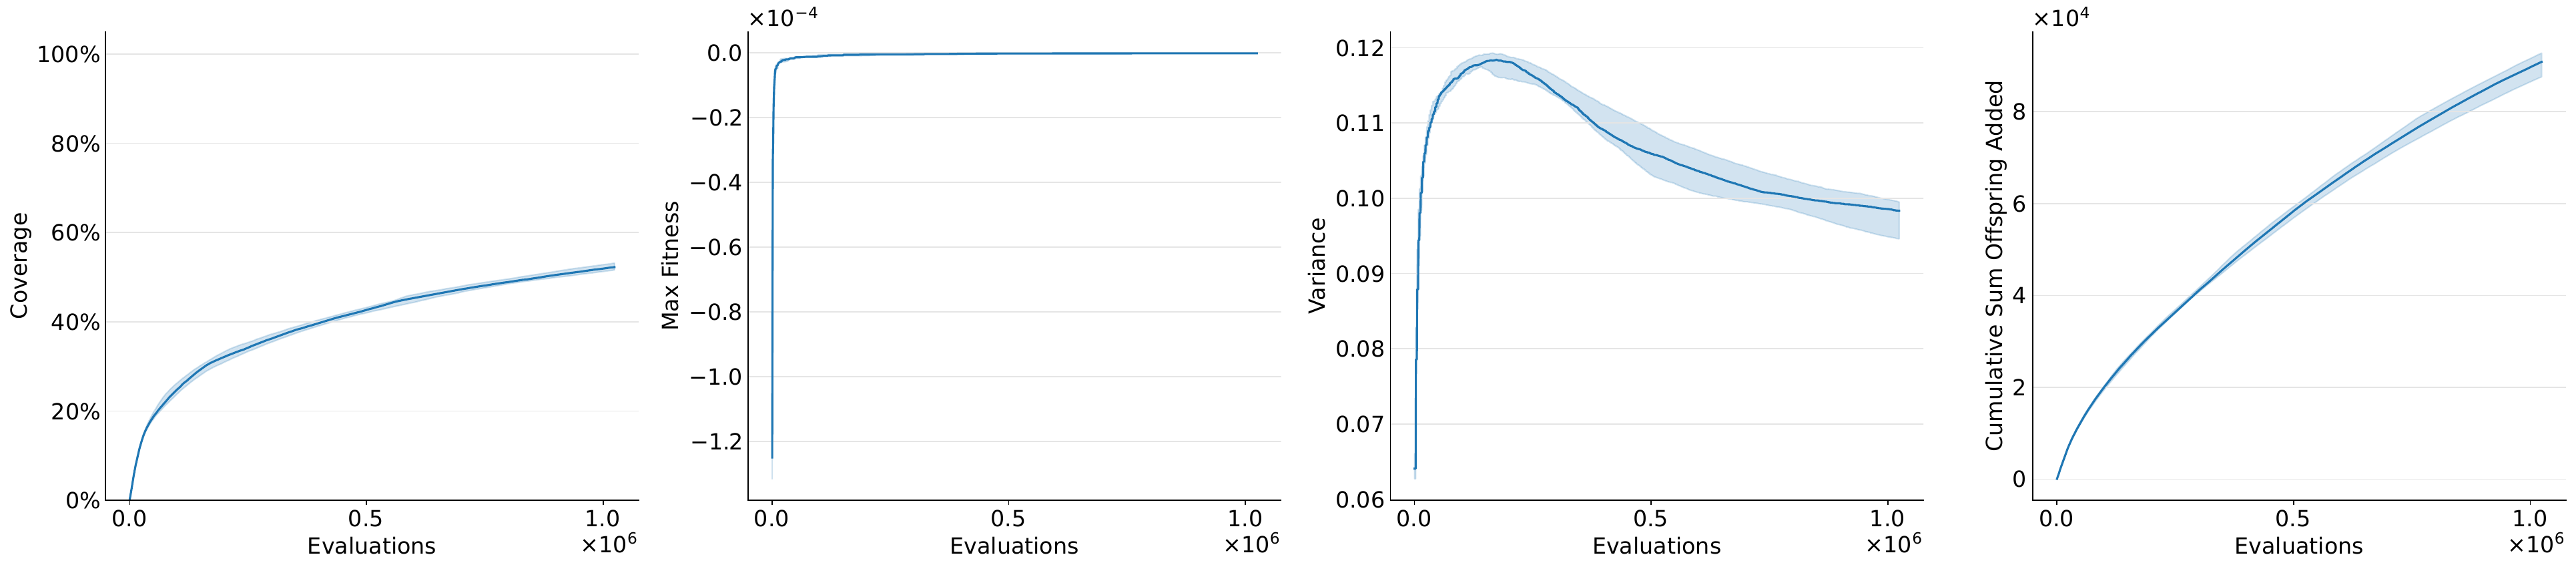}
%     \caption{Entropy, Variance and Cumulative Sum of Offspring Added to the unstructured repertoire for \aurora{} with different fitness functions, including the unsupervised fitness. Each experiment is replicated 20 times with random seeds. The solid line is the median and the shaded area represents the first and third quartiles.}
% \end{figure*}
%
\begin{figure*}[h!]
    \centering
    \includegraphics[width=\textwidth]{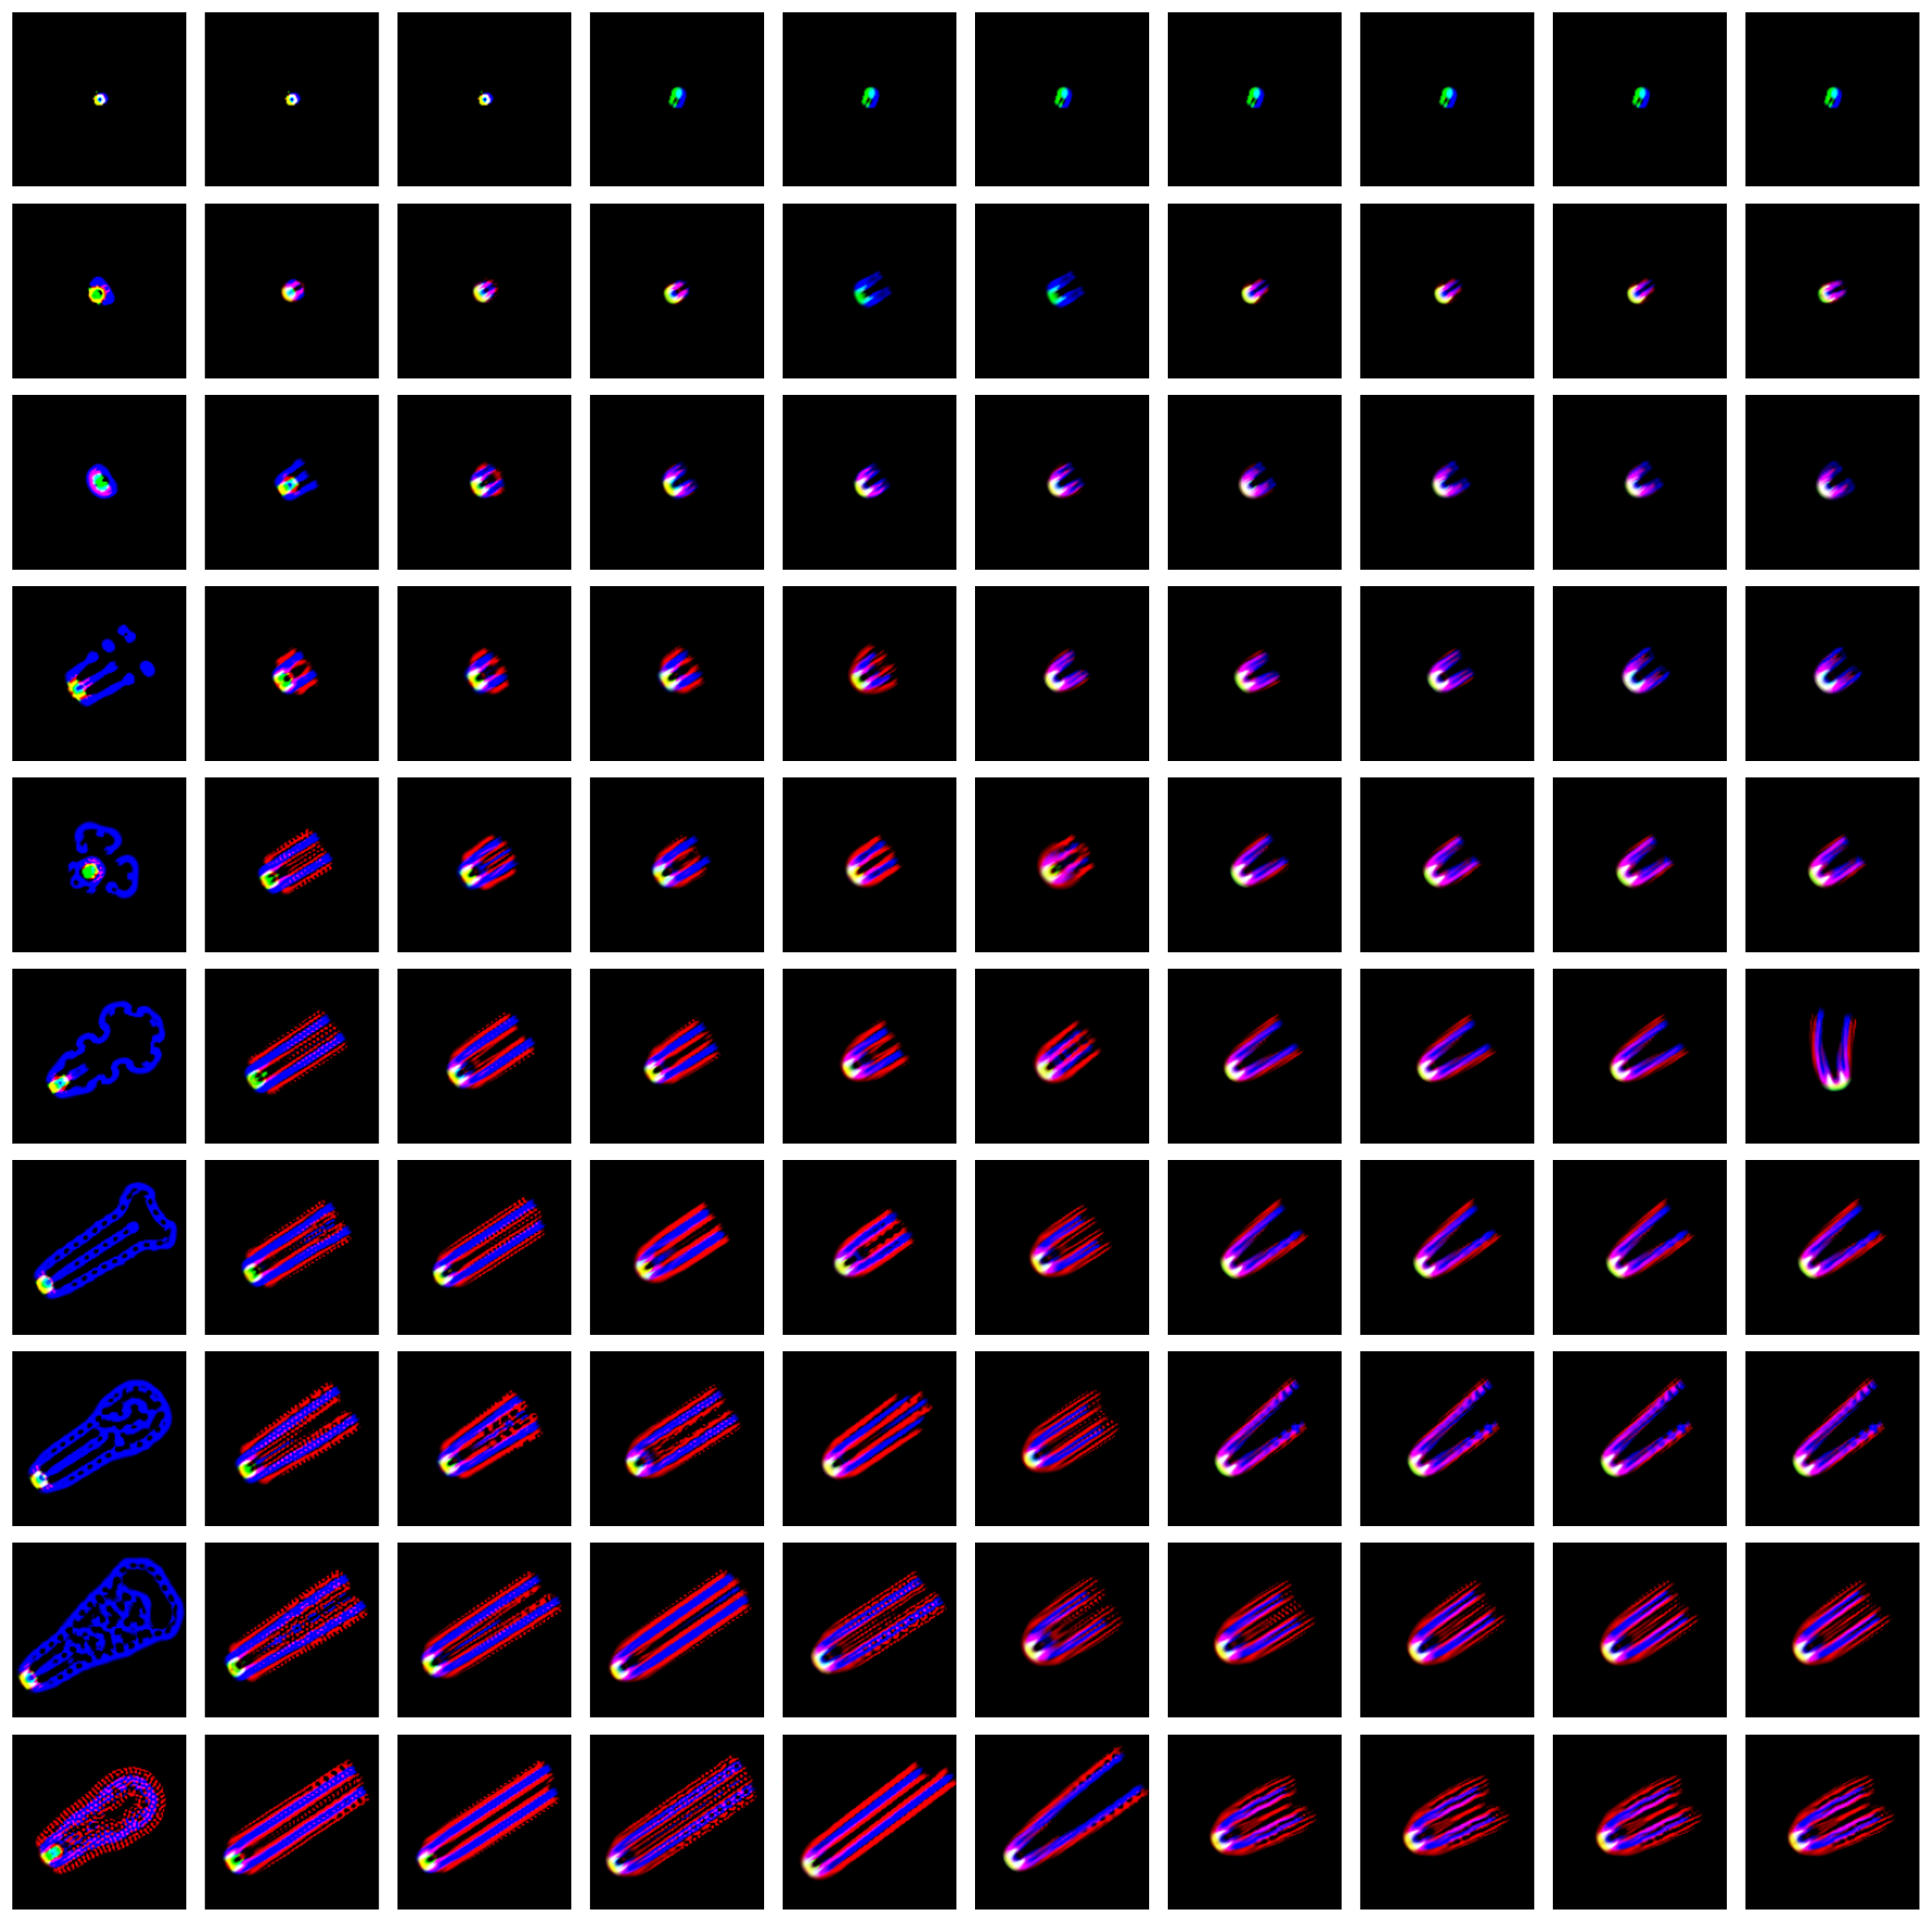}
    \caption{Entropy, Variance and Cumulative Sum of Offspring Added to the unstructured repertoire for \aurora{} with different fitness functions, including the unsupervised fitness. Each experiment is replicated 20 times with random seeds. The solid line is the median and the shaded area represents the first and third quartiles.}
\end{figure*}

% \begin{figure*}[h!]
%     \centering
%     \includegraphics[width=\textwidth]{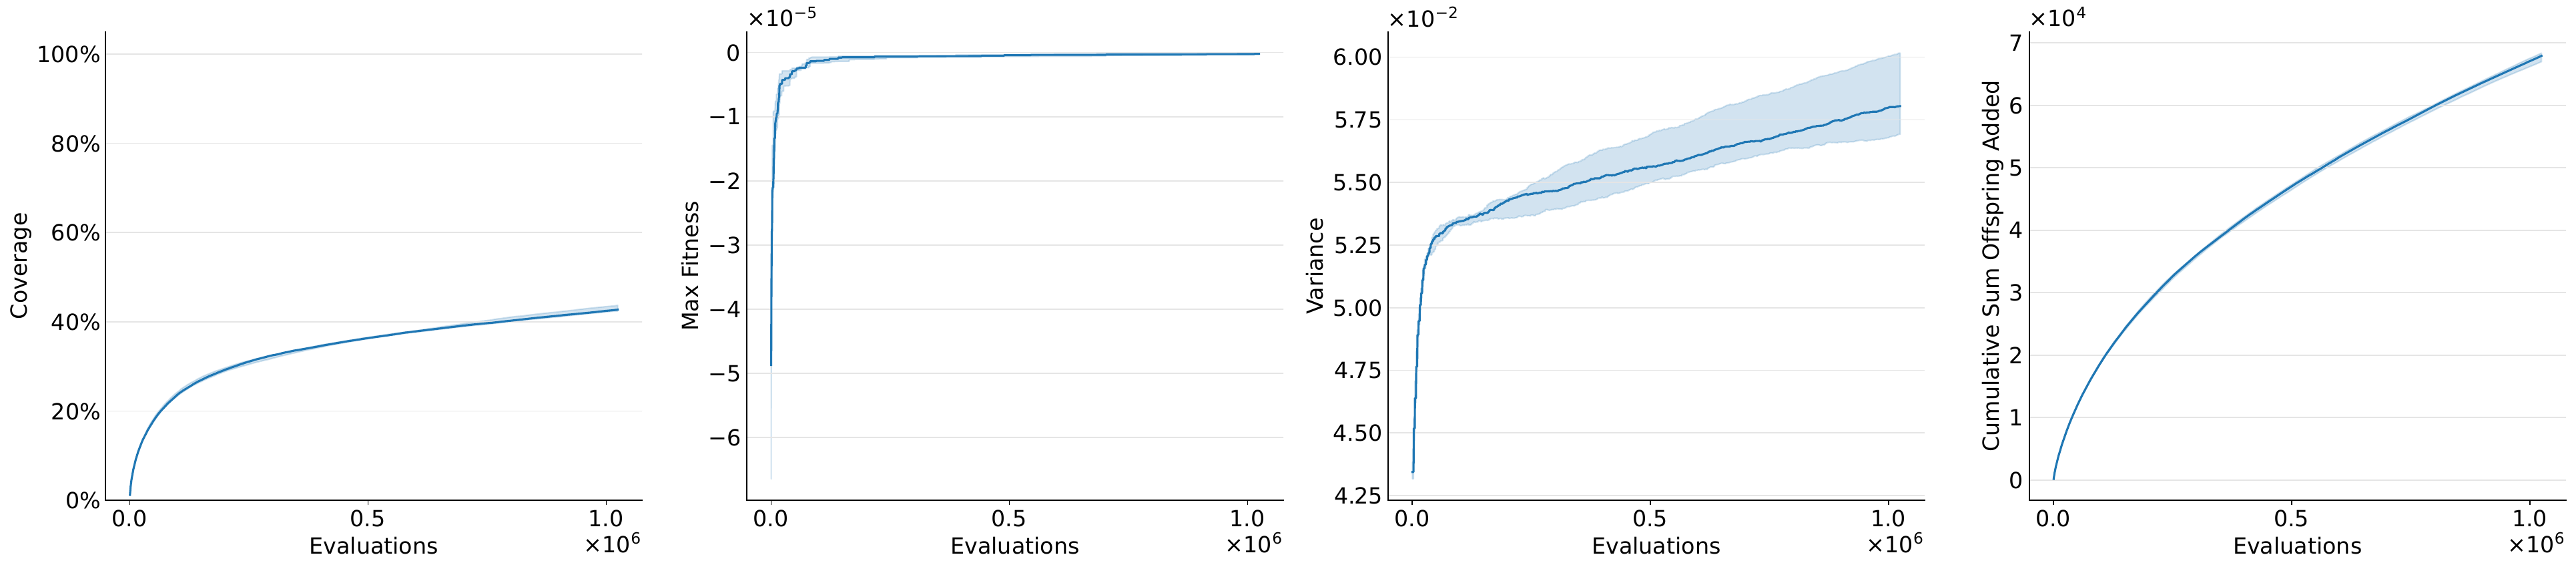}
%     \caption{Entropy, Variance and Cumulative Sum of Offspring Added to the unstructured repertoire for \aurora{} with different fitness functions, including the unsupervised fitness. Each experiment is replicated 20 times with random seeds. The solid line is the median and the shaded area represents the first and third quartiles.}
% \end{figure*}
%
\begin{figure*}[h!]
    \centering
    \includegraphics[width=\textwidth]{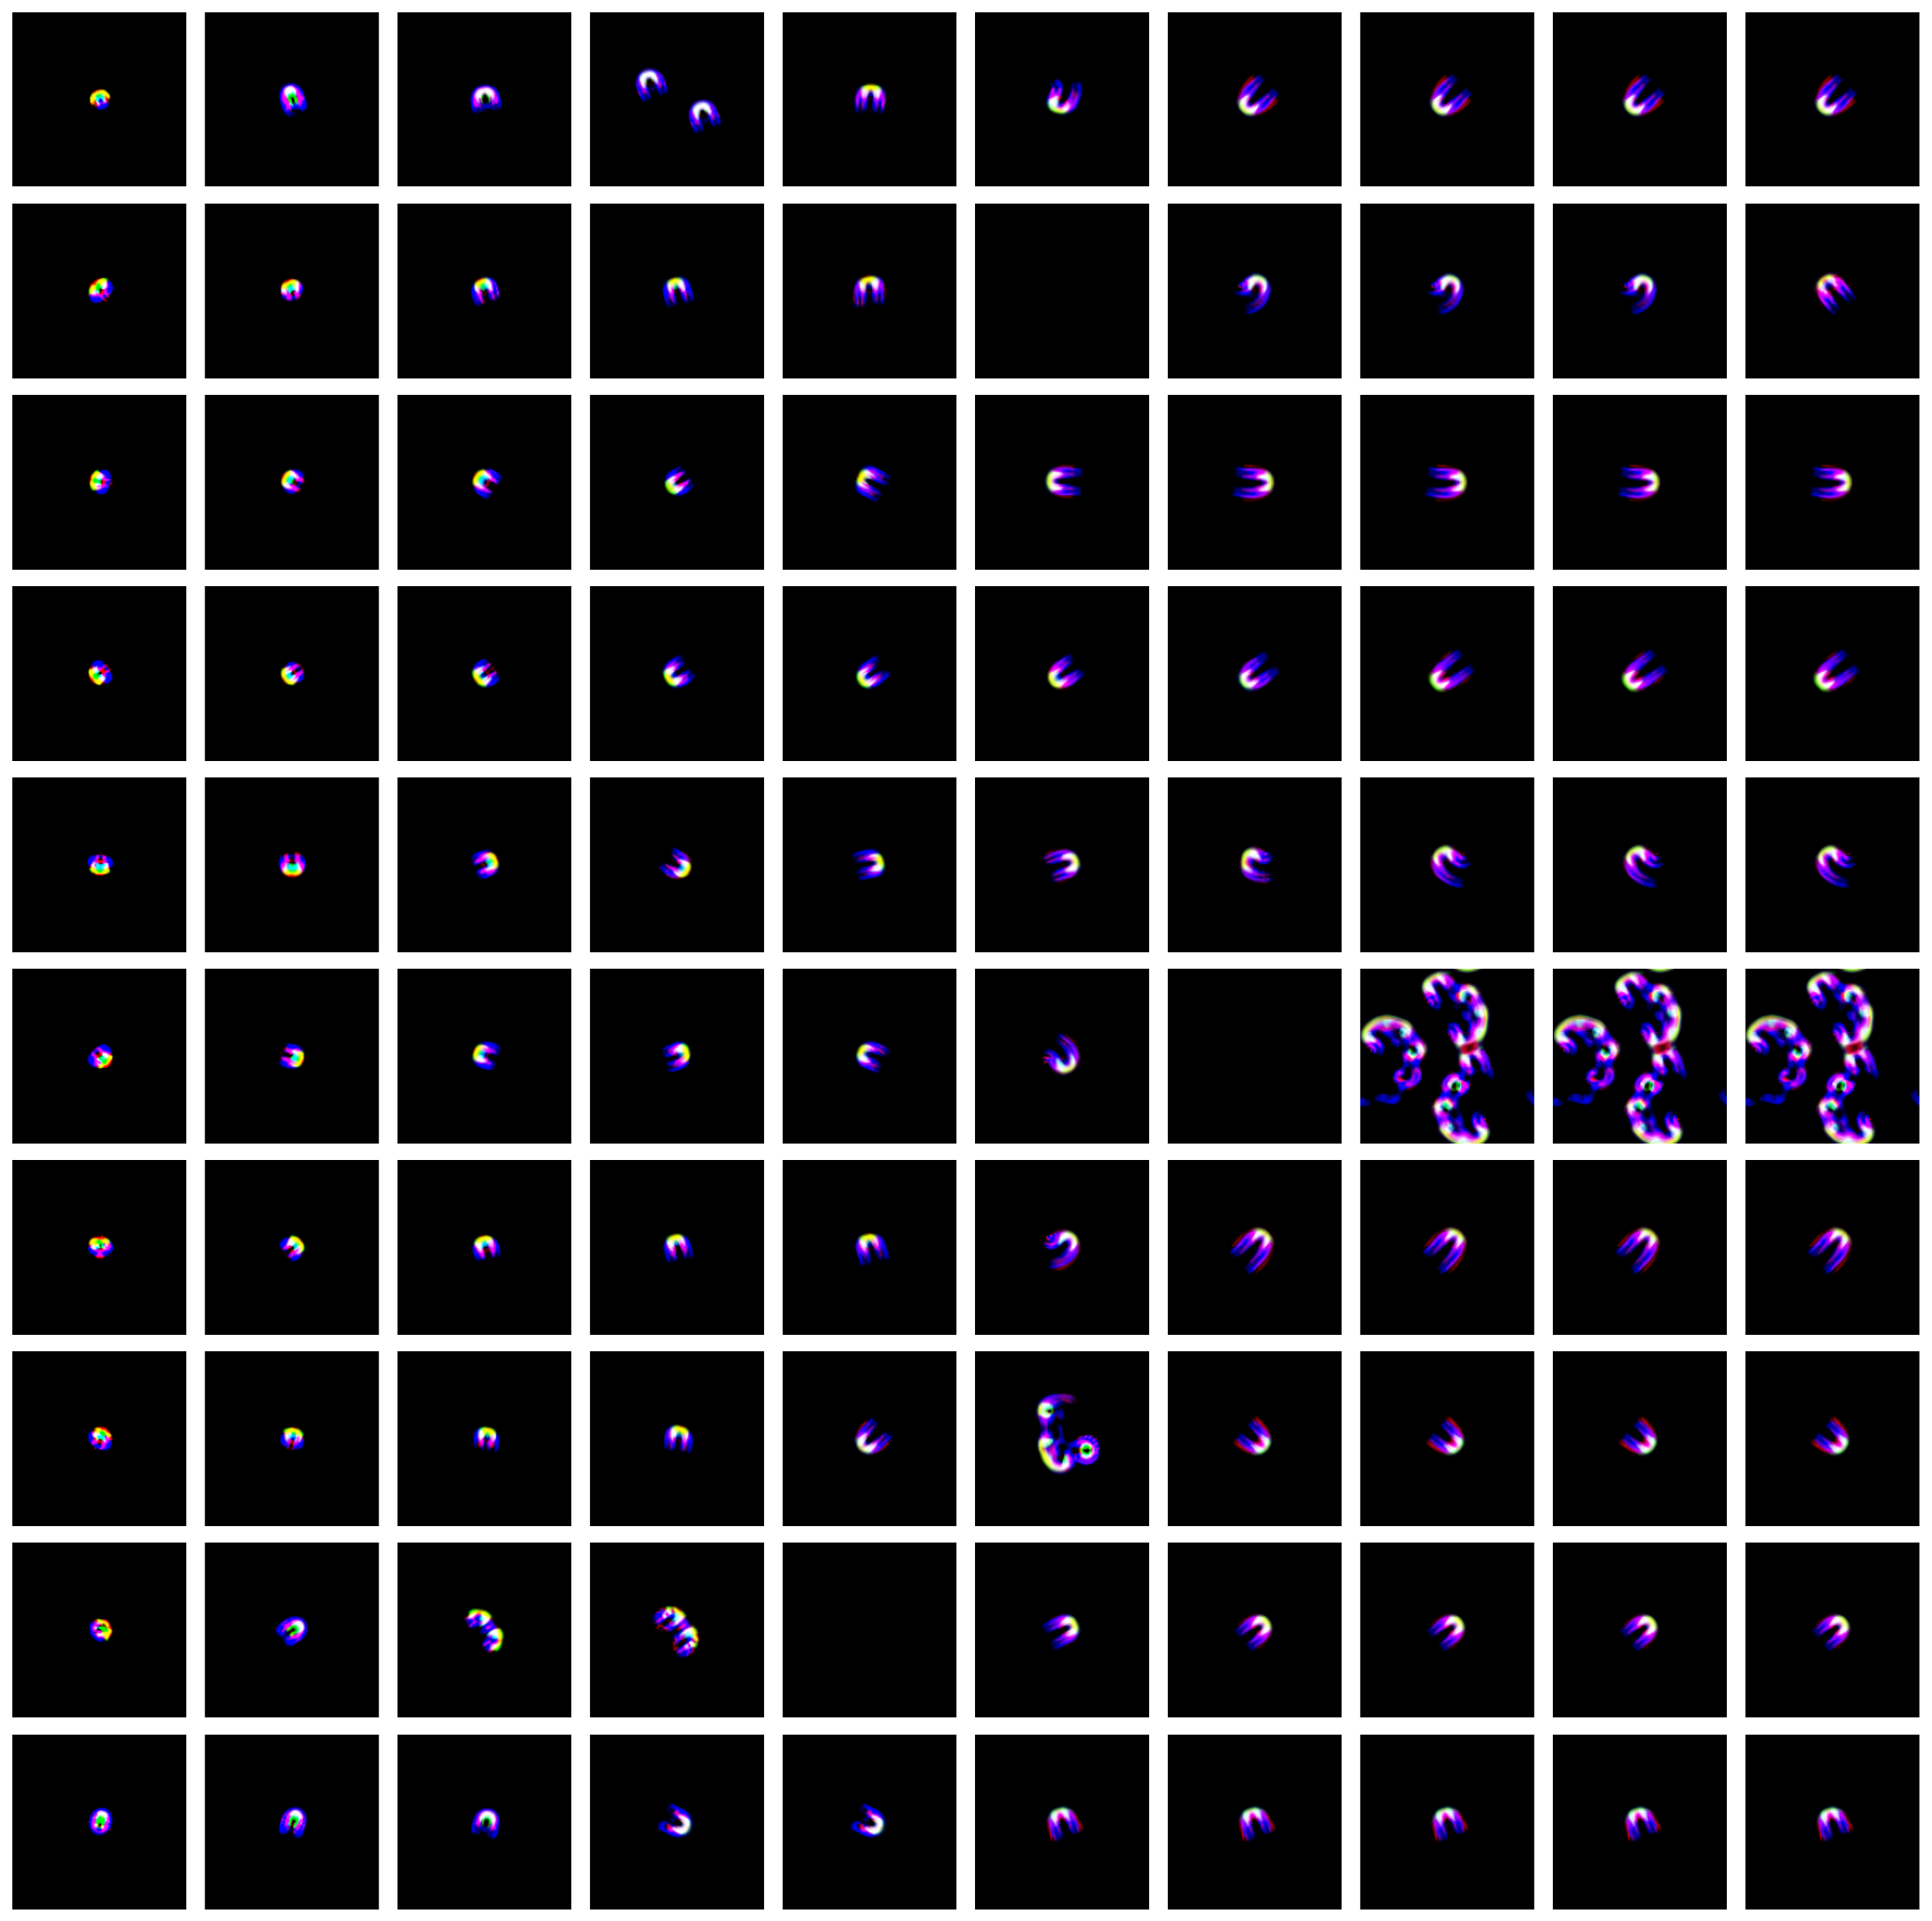}
    \caption{Entropy, Variance and Cumulative Sum of Offspring Added to the unstructured repertoire for \aurora{} with different fitness functions, including the unsupervised fitness. Each experiment is replicated 20 times with random seeds. The solid line is the median and the shaded area represents the first and third quartiles.}
\end{figure*}
