# Supplementary material for: Toward Artificial Open-Ended Evolution within Lenia using Quality-Diversity
Source: arXiv:2406.04235 source file (2024-06-06)
Supplement: Supplementary file 2 [file 2_hyperparameters.tex]

\newpage
\section{Hyperparameters}
\subsection{Lenia simulation}
\begin{table}[h!]
\label{tab:hyperparameters-lenia}
\caption{Lenia hyperparameters}
\centering
\begin{tabular}{l | c}
\toprule
Parameter & Value\\
\midrule
Space resolution $R$ & $12$\\
Time resolution $T$ & $2$\\
Number of dimensions $d$ & $2$\\
Number of channels $c$ & $3$\\
World size & $128 \times 128 \times 3$\\
World scale & $1$\\
Number of steps $N$ & $200$\\
\bottomrule
\end{tabular}
\end{table}

\subsection{\me}
\begin{table}[h!]
\label{tab:hyperparameters-me}
\caption{\me{} hyperparameters}
\centering
\begin{tabular}{l | c}
\toprule
Parameter & Value\\
\midrule
Number of generations & $4000$\\
Batch size & $256$\\
Repertoire size & $32,768$\\
\hline
GA isoline $\sigma_1$ & $0.005$\\
GA isoline $\sigma_2$ & $0.05$\\
\hline
Discard $n$ & $50$\\
$m_\text{min}$ & $0.1$\\
$m_\text{max}$ & $\infty$\\
\bottomrule
\end{tabular}
\end{table}

\subsection{\aurora}
\begin{table}[h!]
\label{tab:hyperparameters-aurora}
\caption{\aurora{} hyperparameters}
\centering
\begin{tabular}{l | c}
\toprule
Parameter & Value\\
\midrule
Number of generations & $4000$\\
Batch size & $256$\\
Repertoire size & $32,768$\\
\hline
GA isoline $\sigma_1$ & $0.005$\\
GA isoline $\sigma_2$ & $0.05$\\
\hline
Latent size & $8$\\
Number of features & $64$\\
Learning rate & $5 \times 10^{-4}$\\
Batch size & $256$\\
\hline
Discard $n$ & $184$\\
$m_\text{min}$ & $0.1$\\
$m_\text{max}$ & $4$\\
\bottomrule
\end{tabular}
\end{table}
